# Supplementary material for: Attacking the DeFi Ecosystem with Flash Loans for Fun and Profit
Source: arXiv:2003.03810 source file (2021-03-20)
Supplement: Supplementary file 1 [file appendix.tex]

\section{Contract Project Map}\label{app:map}

Mapping of smart contract addresses to project name used to classify flash loan usages.
\begin{lstlisting}[basicstyle=\tiny]
category_map = {
    "0x6B175474E89094C44Da98b954EedeAC495271d0F": "Dai",
    "0x61935CbDd02287B511119DDb11Aeb42F1593b7Ef": "0x",
    "0x197E90f9FAD81970bA7976f33CbD77088E5D7cf7": "MakerDAO",
    "0x7a3370075a54B187d7bD5DceBf0ff2B5552d4F7D": "Kyber",
    "0x9759A6Ac90977b93B58547b4A71c78317f391A28": "MakerDAO",
    "0xad37fd42185Ba63009177058208dd1be4b136e6b": "MakerDAO",
    "0x2a1530C4C41db0B0b2bB646CB5Eb1A67b7158667": "Uniswap",
    "0x398eC7346DcD622eDc5ae82352F02bE94C62d119": "Aave",
    "0x3d9819210A31b4961b30EF54bE2aeD79B9c9Cd3B": "Compound",
    "0x5d3a536E4D6DbD6114cc1Ead35777bAB948E3643": "cDai",
    "0xc0829421C1d260BD3cB3E0F06cfE2D52db2cE315": "Bancor",
    "0x8007aa43792A392b221DC091bdb2191E5fF626d1": "Kyber",
    "0x5bcA0f6cD5F9a74895d66005acEf969342F301A0": "CollateralSwap",
    "0x20a1d01e03D65495AE157d47E4519EceACb608f6": "OneLeverage",
    "0x5ef30b9986345249bc32d8928B7ee64DE9435E39": "MakerDAO",
    "0x3D0B1912B66114d4096F48A8CEe3A56C231772cA": "MakerDAO",
    "0x3Ab6564d5c214bc416EE8421E05219960504eeAD": "Bancor",
    "0x201b704Ae89b31fB795F5EF41E62461b9302E1BA": "DSProxy",
    "0x65bF64Ff5f51272f729BDcD7AcFB00677ced86Cd": "Kyber",
    "0x4Ddc2D193948926D02f9B1fE9e1daa0718270ED5": "cEther",
    "0x2F0b23f53734252Bda2277357e97e1517d6B042A": "MakerDAO",
    "0x23401C7811411f40008CE9688EdB293D8fe507bc": "DSProxy",
    "0x06f7Bf937Dec0C413a2E0464Bb300C4d464bb891": "Bancor",
    "0x3dfd23A6c5E8BbcFc9581d2E864a68feb6a076d3": "Aave",
    "0x63825c174ab367968EC60f061753D3bbD36A0D8F": "Kyber",
    "0x794e6e91555438aFc3ccF1c5076A74F42133d08D": "Oasis",
    "0xC9A4AEF09fD9ae835A0c60A0757C8dd748116781": "OneLeverage",
    "0x1F573D6Fb3F13d689FF844B4cE37794d79a7FF1C": "Bancor",
    "0xFa8C4B17ac43A025977F5feD843B6c8c4EA52F1c": "DSProxy",
    "0x2E642b8D59B45a1D8c5aEf716A84FF44ea665914": "Uniswap",
    "0xE03374cAcf4600F56BDDbDC82c07b375f318fc5C": "Bancor",
    "0x309627af60F0926daa6041B8279484312f2bf060": "Bancor",
    "0x09cabEC1eAd1c0Ba254B09efb3EE13841712bE14": "Uniswap",
    "0x0D8775F648430679A709E98d2b0Cb6250d2887EF": "BAT",
    "0x207737F726c13C1298B318D233AAa6164EE6b712": "DSProxy",
    "0x818E6FECD516Ecc3849DAf6845e3EC868087B755": "Kyber",
    "0x35D1b3F3D7966A1DFe207aa4514C12a259A0492B": "MakerDAO",
    "0x39755357759cE0d7f32dC8dC45414CCa409AE24e": "Oasis",
    "0xA0b86991c6218b36c1d19D4a2e9Eb0cE3606eB48": "USDC",
    "0xC02aaA39b223FE8D0A0e5C4F27eAD9083C756Cc2": "WETH9",
    "0x7778d1011e19C0091C930d4BEfA2B0e47441562A": "OneLeverage",
    "0x89d24A6b4CcB1B6fAA2625fE562bDD9a23260359": "SAI",
    "0xd3ec78814966Ca1Eb4c923aF4Da86BF7e6c743bA": "Bancor",
    "0x19c0976f590D67707E62397C87829d896Dc0f1F1": "MakerDAO",
    "0x35A679A2A63F774BBEc5E80E32aE436BC3b5d98e": "DSProxy",
}
\end{lstlisting}
